# Supplementary material for: Flowette: Flow Matching with Graphette Priors for Graph Generation
Source: arXiv:2602.23566 source file (2026-11-06)
Supplement: Supplementary file 1 [file 10_appendix.tex]

\section{Extended discussion of limitations}
\label{sec:extended-limitations}

We expand here on each of the four limitations summarised in the \emph{Observed limitations} paragraph of Section~\ref{sec:results-or-wherever}.

\paragraph{Computational cost of FGW coupling.}
Fused Gromov-Wasserstein coupling between batches of $B$ graphs of up to $n$ nodes carries an $\mathcal{O}(B^2 n^3)$ cost, dominated by the inner alignment problem. In practice this is precomputed once per dataset on the training split alone (avoiding any leakage from validation or test samples) and reused across epochs, keeping total training time within a small constant factor of comparable diffusion- and flow-based baselines (Table~\ref{tab:runtime}). However, the cubic dependence on graph size means Flowette is most appropriate for graphs with up to a few hundred nodes; scaling to substantially larger graphs would likely require approximate FGW solvers or sparser couplings, which we leave for future work.

\paragraph{Choice of graph edit function.}
Graphettes are designed so that the choice of graph edit function $f$ requires only coarse, qualitative knowledge of the target family --- whether it contains rings (GEF~3), hubs or stars (GEF~4), requires acyclicity (GEF~2), or has no dominant motif (the identity GEF~1). For the benchmarks evaluated here, this choice is answerable from basic dataset statistics. Where such knowledge is unavailable a priori, the framework currently does not provide a data-driven mechanism for selecting $f$, although the small discrete menu of edit functions makes brute-force selection plausible. Automating this choice --- for example by learning the edit function jointly with the velocity field, or by selecting it from data via motif statistics --- is a natural direction for future work.

\paragraph{Domain-specific regularisation.}
The chemistry-aware terms $\mathcal{L}_\mathrm{val}$ and $\mathcal{L}_\mathrm{atom}$ encode molecular feasibility constraints (valence satisfaction and atom-type marginal matching) and are therefore restricted to molecular benchmarks. They are absent on the synthetic benchmarks (Tree, SBM, Ego-small), where Flowette still attains $100\%$ V.U.N.\ on Tree and SBM, demonstrating that the core framework --- FGW coupling, graphette priors, endpoint-consistency regularisation, and the GNN-based velocity transformer --- produces strong structural fidelity without any domain-specific terms. Whether analogous regularisers would benefit other complex domains (e.g.\ biological networks with stoichiometric constraints, or program graphs with type constraints) is left to future work.

\paragraph{Discrete projection at generation.}
Because Flowette operates on continuous relaxations of adjacency and edge-feature tensors, generation requires a final discrete projection step: argmax decoding for atom and bond types, and symmetrisation followed by valence-aware pruning for adjacency (Appendix~\ref{sec:projection-or-wherever}). This deterministic post-processing applies only at inference and does not affect training or gradient flow, but introduces a small gap between the integrated continuous trajectory and the final discrete graph. This is a well-known property of continuous-relaxation graph generative models and is not specific to Flowette.
